# Supplementary material for: MIM4DD: Mutual Information Maximization for Dataset Distillation
Source: arXiv:2312.16627 source file (2023-12-27)
Supplement: Supplementary file 1 [file supp_neurips.tex]

\documentclass{article}

% if you need to pass options to natbib, use, e.g.:
%     \PassOptionsToPackage{numbers, compress}{natbib}
% before loading neurips_2021

\usepackage{natbib}
\PassOptionsToPackage{numbers, compress}{natbib}

% ready for submission
\usepackage{neurips_2021}

% to compile a preprint version, e.g., for submission to arXiv, add add the
% [preprint] option:
    % \usepackage[preprint]{neurips_2021}

% to compile a camera-ready version, add the [final] option, e.g.:
    % \usepackage[final]{neurips_2021}

% to avoid loading the natbib package, add option nonatbib:
    % \usepackage[nonatbib]{neurips_2021}
\usepackage[breaklinks=true,bookmarks=false]{hyperref}

\usepackage[utf8]{inputenc} % allow utf-8 input
\usepackage[T1]{fontenc}    % use 8-bit T1 fonts
\usepackage{hyperref}       % hyperlinks
\usepackage{url}            % simple URL typesetting
\usepackage{booktabs}       % professional-quality tables
\usepackage{amsfonts}       % blackboard math symbols
\usepackage{nicefrac}       % compact symbols for 1/2, etc.
\usepackage{microtype}      % microtypography
\usepackage{multicol}
\usepackage{amsmath}
\usepackage{enumitem}
\usepackage{amssymb}
\usepackage{wrapfig}
\usepackage{xcolor}
\usepackage{multirow}
\usepackage{float}
\usepackage{graphicx}
\usepackage[position=top]{subfig}
\usepackage{algpseudocode}  
\usepackage{algorithmicx,algorithm}
\usepackage{caption}

\hypersetup{
	colorlinks=true,
% 	linkcolor=cyan,
% 	filecolor=blue,      
% 	urlcolor=red,
% 	citecolor=black,
}

\title{LCR-BNN: Lipschitz Continuity Retention for Accurate Binary Neural Networks}
% \title{Smoothing Binary Neural Networks with Lipschitz Continuity}

% The \author macro works with any number of authors. There are two commands
% used to separate the names and addresses of multiple authors: \And and \AND.
%
% Using \And between authors leaves it to LaTeX to determine where to break the
% lines. Using \AND forces a line break at that point. So, if LaTeX puts 3 of 4
% authors names on the first line, and the last on the second line, try using
% \AND instead of \And before the third author name.

\author{
  \textbf{Yuzhang Shang$^{1}$, Ziliang Zong$^{4}$, }
  \textbf{Dan Xu$^{3}$, Liqiang Nie$^{2}$, Yan Yan$^{1}$} \\
  $^{1}$Department of Computer Science, Illinois Institute of Technology, USA \\ 
  $^{2}$Shandong University, China \\ 
  $^{3}$HKUST, China\\ 
  $^{4}$Texas State University, USA \\
%   \texttt{yzshawn@outlook.com, \{email1, email2,\}@affiliation.edu} \\
  \texttt{yzshawn@outlook.com, nieliqiang@gmail.com, yyan34@iit.edu} 
%   \texttt{} 
}

\begin{document}

\maketitle

\input{0Abstract}
\input{1Intro}
\input{3Method}
\input{4Exp}
\vspace{-3mm}
\input{2Related}
\vspace{-3mm}
\input{5Conclusion}

\clearpage
{\small
\bibliographystyle{unsrt}
\bibliography{references}
}

%%%%%%%%%%%%%%%%%%%%%%%%%%%%%%%%%%%%%%%%%%%%%%%%%%%%%%%%%%%%
